# Supplementary material for: BioLM-Score: Language-Prior Conditioned Probabilistic Geometric Potentials for Protein-Ligand Scoring
Source: arXiv:2602.18476 source file (2026-02-09)
Supplement: Supplementary file 1 [file suppl.pdf]

# Supplementary Information for BioLM-Score: Language-Prior Conditioned Probabilistic Geometric Potentials for Protein–Ligand Scoring

Anonymous

## 1 Supplementary Information A: Detailed Formulations of Graph Encoders

Let  $\mathbf{x}_i$  denote the initial node feature vector and  $\mathbf{a}_{ij}$  the initial edge feature vector. Regardless of the backbone architecture, inputs are projected into continuous embeddings via learnable linear transformations:

$$\mathbf{h}_i^0 = \mathbf{W}_x \mathbf{x}_i, \quad \mathbf{e}_{ij}^0 = \mathbf{W}_a \mathbf{a}_{ij}, \quad (1)$$

where  $\mathbf{h}_i, \mathbf{e}_{ij} \in \mathbb{R}^d$ . We investigate two distinct graph encoding architectures to iteratively update these representations over  $L$  layers.

### GatedGCN Backbone

We adopt the Gated Graph Convolutional Network (GatedGCN) as our primary encoder. Formally, let  $\mathbf{h}_i^\ell \in \mathbb{R}^d$  and  $\mathbf{e}_{ij}^\ell \in \mathbb{R}^d$  denote the features of node  $i$  and edge  $(i, j)$  at the  $\ell$ -th layer, respectively. We first compute the *intermediate edge feature*  $\tilde{\mathbf{e}}_{ij}^\ell$  as:

$$\tilde{\mathbf{e}}_{ij}^\ell = W_C^\ell \mathbf{h}_i^\ell + W_D^\ell \mathbf{h}_j^\ell + W_E^\ell \mathbf{e}_{ij}^\ell, \quad (2)$$

where  $W_C^\ell, W_D^\ell, W_E^\ell \in \mathbb{R}^{d \times d}$  are learnable weight matrices. Subsequently, we derive the edge gating vector  $g_{ij}^\ell \in \mathbb{R}^d$  via a normalization over the neighborhood  $\mathcal{N}_i$ :

$$g_{ij}^\ell = \frac{\sigma(\tilde{\mathbf{e}}_{ij}^\ell)}{\sum_{k \in \mathcal{N}_i} \sigma(\tilde{\mathbf{e}}_{ik}^\ell) + \varepsilon}, \quad (3)$$

where  $\sigma(\cdot)$  is the sigmoid function and  $\varepsilon$  is a small constant for numerical stability.

We define a composite update function  $\phi(\mathbf{z}) = \text{Dropout}(\omega(\text{BN}(\mathbf{z})))$ , where  $\text{BN}(\cdot)$  denotes Batch Normalization. The activation  $\omega(\cdot)$  is set to SiLU for node features and ReLU for edge features. Finally, the layer updates are defined as:

$$\mathbf{h}_i^{\ell+1} = \mathbf{h}_i^\ell + \phi \left( W_A^\ell \mathbf{h}_i^\ell + \sum_{j \in \mathcal{N}_i} g_{ij}^\ell \odot (W_B^\ell \mathbf{h}_j^\ell) \right), \quad (4)$$

$$\mathbf{e}_{ij}^{\ell+1} = \mathbf{e}_{ij}^\ell + \phi(\tilde{\mathbf{e}}_{ij}^\ell), \quad (5)$$

where  $\odot$  denotes the Hadamard product, and  $W_A^\ell, W_B^\ell \in \mathbb{R}^{d \times d}$  are transformation matrices.

**Structure-aware Graph Transformer (GT).** Alternatively, we employ a Graph Transformer designed to capture dependencies while explicitly modeling edge dynamics. Unlike standard Transformers, our attention mechanism incorporates edge features into the attention score calculation and, conversely, uses attention coefficients to update edge representations.

For each attention head  $k \in \{1, \dots, H\}$  at layer  $\ell$ , we first compute the query, key, value, and edge projections via learnable matrices  $\mathbf{Q}^{k,\ell}, \mathbf{K}^{k,\ell}, \mathbf{V}^{k,\ell}, \mathbf{E}^{k,\ell} \in \mathbb{R}^{d_k \times d}$ , where  $d_k = d/H$ . The structure-aware attention coefficients  $\alpha_{ij}^{k,\ell}$  are computed as:

$$\alpha_{ij}^{k,\ell} = \text{softmax}_j \left( \frac{(\mathbf{Q}^{k,\ell} \mathbf{h}_i^\ell)^\top (\mathbf{K}^{k,\ell} \mathbf{h}_j^\ell) \cdot (\mathbf{E}^{k,\ell} \tilde{\mathbf{e}}_{ij}^\ell)}{\sqrt{d_k}} \right), \quad (6)$$

where  $\tilde{\mathbf{e}}_{ij}^\ell$  represents the edge features for the current layer. Crucially, the attention scores are not only used to aggregate node features but also concatenated to update the edge features, ensuring the edges reflect the interaction strength between nodes:

$$\tilde{\mathbf{h}}_i^{\ell+1} = \mathbf{h}_i^\ell + \mathbf{W}_O^\ell \text{Dropout} \left( \left\|_{k=1}^H \left( \sum_{j \in \mathcal{N}_i} \alpha_{ij}^{k,\ell} \mathbf{V}^{k,\ell} \mathbf{h}_j^\ell \right) \right\| \right), \quad (7)$$

$$\tilde{\mathbf{e}}_{ij}^{\ell+1} = \mathbf{e}_{ij}^\ell + \mathbf{W}_E^\ell \text{Dropout} \left( \left\|_{k=1}^H \alpha_{ij}^{k,\ell} \right\| \right), \quad (8)$$

where  $\|$  denotes concatenation of  $H$  heads. Finally, both node and edge features undergo a feed-forward transition with residual connections:

$$\mathbf{h}_i^{\ell+1} = \tilde{\mathbf{h}}_i^{\ell+1} + \mathbf{W}_{h2}^\ell \text{Dropout} \left( \text{SiLU} \left( \mathbf{W}_{h1}^\ell \text{BN}(\tilde{\mathbf{h}}_i^{\ell+1}) \right) \right), \quad (9)$$

$$\mathbf{e}_{ij}^{\ell+1} = \tilde{\mathbf{e}}_{ij}^{\ell+1} + \mathbf{W}_{e2}^\ell \text{Dropout} \left( \text{SiLU} \left( \mathbf{W}_{e1}^\ell \text{BN}(\tilde{\mathbf{e}}_{ij}^{\ell+1}) \right) \right). \quad (10)$$

This formulation ensures a joint optimization process where edge features dynamically adapt to the node interaction context.

## 2 Supplementary Information B: Implementation Details

**Dataset Preparation.** We utilize the PDBBind v2020 dataset for training and validation, while designating CASF-2016 as the independent test set. The protein structures undergo standard preprocessing via the RTMScore pipeline, including water removal, hydrogenation, bond order assignment, and hydrogen bond network optimization. Subsequently, energy minimization is performed using the OPLS-3 force field with harmonic restraints ( $\text{RMSD} < 0.3 \text{ \AA}$ ) to refine the structures. After filtering out complexes with parsing failures (via RDKit valence checks), we obtain 19,300 valid samples. To strictly prevent data leakage, we remove any complexes overlapping with the CASF-2016 benchmark based on PDB IDs, resulting in a final dataset of 19,015 complexes. This set is randomly partitioned into 17,515 samples for training and 1,500 for validation.

**Model Configuration and Training.** The structural encoder is configured with  $N = 6$  GatedGCN layers and a hidden dimension of  $d = 128$ . For interaction modeling, the MDN hidden size is set to 128 with  $K = 10$  mixture components. To mitigate overfitting, we apply a dropout rate of 0.15. The model is optimized using the Adam optimizer for a maximum of 2,000 epochs, with early stopping triggered if the validation loss does not improve for 70 consecutive epochs. The initial learning rate is set to  $5 \times 10^{-4}$  and weight decay to  $1 \times 10^{-5}$ . The auxiliary loss weights are set to  $\lambda_{\text{atom}} = \lambda_{\text{bond}} = 0.1$ .

**Molecular Docking Protocol.** Leveraging the predictive capability of BioLM-Score, we establish a scoring-guided docking framework, termed BSDock, and benchmark it on the PDBBind Coreset. The ligand conformation is parameterized as a vector  $\mathbf{x} \in \mathbb{R}^D$ , comprising three components: (i) global orientation represented by Euler angles, (ii) relative translation in 3D Euclidean space, and (iii) torsion angles for all rotatable bonds.

We employ Differential Evolution (DE) to perform a global search over these conformational variables, initializing from random conformations and utilizing BioLM-Score as the objective function. The DE hyperparameters are configured as follows: a population size of  $8 \times D$ , a maximum of 500 iterations, a crossover rate ( $CR$ ) of 0.8, and a mutation factor ( $F$ ) randomly sampled from  $[0.5, 1]$ . To bridge the granularity gap between our residue-atom distance constraints and the fine-grained atom-atom potentials required for precise binding, we introduce a post-hoc local refinement stage. Specifically, the candidate conformations identified by the global DE search undergo local optimization via AutoDock Vina to resolve steric clashes and refine local geometry. This two-stage protocol is denoted as BSDock (optimized) in our experimental results.

### 3 Supplementary Information C: Evaluation Protocol and Metrics

BioLM-Score is evaluated on the CASF-2016 benchmark across four complementary tasks: scoring, ranking, docking, and screening.

**Scoring.** The scoring task assesses the correlation between predicted scores and experimental binding affinities. We report the Pearson correlation coefficient ( $R_p$ ), defined as:

$$R_p = \frac{\sum_{i=1}^n (x_i - \bar{x})(y_i - \bar{y})}{\sqrt{\sum_{i=1}^n (x_i - \bar{x})^2} \sqrt{\sum_{i=1}^n (y_i - \bar{y})^2}}, \quad (11)$$

where  $x_i$  and  $y_i$  denote the predicted and experimental affinities, respectively, and  $\bar{x}$  and  $\bar{y}$  represent their means over  $n$  samples.

**Ranking.** Ranking evaluates the model’s capability to preserve the relative order of binding affinities among ligands targeting the same protein. We utilize the CASF-2016 benchmark, which consists of 57 target groups, each containing  $n = 5$  ligand-protein complexes. For each target group  $t$ , we compute the Spearman correlation coefficient ( $\rho_t$ ) between the predicted and experimental rankings. Let  $r_{x,i}$  and  $r_{y,i}$  denote the rank of the  $i$ -th complex based on predicted and experimental affinities, respectively. The coefficient  $\rho_t$  is calculated as the Pearson correlation of these rank variables:

$$\rho_t = \frac{\sum_{i=1}^n (r_{x,i} - \bar{r}_x)(r_{y,i} - \bar{r}_y)}{\sqrt{\sum_{i=1}^n (r_{x,i} - \bar{r}_x)^2} \sqrt{\sum_{i=1}^n (r_{y,i} - \bar{r}_y)^2}}, \quad (12)$$

where  $\bar{r}_x$  and  $\bar{r}_y$  represent the mean ranks, and  $n = 5$  is the number of samples within the cluster. The final ranking score is the average correlation across all targets:

$$R_s = \frac{1}{57} \sum_{t=1}^{57} \rho_t. \quad (13)$$

**Docking.** The docking task evaluates the model’s ability to prioritize near-native poses. We utilize the Top-1 Success Rate ( $SR_1$ ) as the primary metric. For each complex, candidate poses are ranked by predicted score in descending order, and the top-ranked pose is selected. A docking attempt is considered successful if the heavy-atom RMSD relative to the crystal structure is less than 2.0 Å.  $SR_1$  is computed as the fraction of successes over all complexes. RMSD is defined as:

$$\text{RMSD} = \sqrt{\frac{1}{N} \sum_{j=1}^N (\mathbf{p}_j - \mathbf{p}_j^*)^2}, \quad (14)$$

where  $\mathbf{p}_j$  and  $\mathbf{p}_j^*$  represent the 3D coordinates of the  $j$ -th heavy atom in the predicted and crystal poses, respectively, and  $N$  is the total number of heavy atoms. To assess the impact of native pose availability,  $SR_1$  is reported under both native-pose-excluded and native-pose-included settings.

**Screening (CASF-2016).** The screening task on CASF-2016 evaluates the ability to distinguish true binders from decoys (forward screening) or identify true targets (reverse screening). In forward screening, the Enrichment Factor (EF) and Success Rate (SR) are reported for the top 1% of candidates. The Enrichment Factor is defined as:

$$EF_{\gamma} = \frac{NTB_{\gamma}}{NTB_{total} \times \gamma}, \quad (15)$$

where  $NTB_{\gamma}$  represents the number of true binders found in the top  $\gamma$  percentile, and  $NTB_{total}$  is the total number of true binders. For reverse screening, we report the Top-1% SR, defined as the fraction of ligands for which the true target appears in the top 1% of ranked proteins.

**Virtual Screening (DEKOIS 2.0).** For the external DEKOIS 2.0 benchmark, we employ metrics that focus on both global discrimination and early enrichment performance.

- **AUROC:** The Area Under the ROC Curve is used to quantify the model’s overall ability to distinguish actives from decoys across the entire ranked list.
- **Early Enrichment Metrics:** To strictly evaluate the model’s utility in identifying hits at the very top of the ranking list, we report the Enrichment Factors at strict cutoffs:  $EF_{0.5\%}$ ,  $EF_{1\%}$ , and  $EF_{5\%}$ . Additionally, we utilize the Boltzmann-Enhanced Discrimination of ROC (BEDROC) score with  $\alpha = 80.5$ , a metric specifically designed to weigh early recognition performance heavily.

Table 1: Performance Comparison of BioLM-Score and Representative Scoring Functions on the CASF-2016 Benchmark

| Methods                        | Scoring      | Ranking      | Docking                           |                                   | Screening                       |                                 |              |
|--------------------------------|--------------|--------------|-----------------------------------|-----------------------------------|---------------------------------|---------------------------------|--------------|
|                                | $R_p$        | $R_s$        | $SR_1$<br>(native poses excluded) | $SR_1$<br>(native poses included) | Forward Screening<br>$EF_{1\%}$ | Reverse screening<br>$SR_{1\%}$ |              |
| AutoDock Vina                  | 0.604        | 0.528        | 0.846                             | 0.902                             | 7.70                            | 0.298                           | 0.137        |
| ChemPLP@GOLD                   | 0.614        | 0.633        | 0.832                             | 0.860                             | 11.91                           | 0.351                           | 0.165        |
| GlideScore-SP                  | 0.513        | 0.419        | 0.846                             | 0.877                             | 11.44                           | 0.368                           | 0.175        |
| $\Delta_{vina} RF_{20}$        | 0.739        | 0.635        | 0.849                             | 0.891                             | 12.36                           | 0.456                           | —            |
| OnionNet-SFCT+Vina             | 0.428        | 0.393        | —                                 | 0.937                             | 15.50                           | 0.421                           | —            |
| PIGNet                         | 0.761        | 0.682        | —                                 | 0.87                              | 19.6                            | 0.554                           | —            |
| PIGNet2                        | 0.747        | 0.651        | —                                 | 0.930                             | 24.90                           | 0.667                           | —            |
| DeepDock                       | 0.460        | 0.425        | —                                 | 0.891                             | 16.40                           | 0.439                           | —            |
| RTMScore                       | 0.456        | 0.539        | 0.93                              | 0.961                             | 25.63                           | 0.596                           | 0.361        |
| GenScore(GT_0)                 | 0.459        | 0.544        | 0.926                             | 0.963                             | 25.54                           | 0.585                           | <b>0.372</b> |
| GenScore(GT_1.0)               | 0.819        | 0.714        | 0.909                             | 0.933                             | 18.76                           | 0.573                           | 0.157        |
| GenScore(GT_ft_1.0)            | 0.798        | 0.67         | 0.93                              | 0.957                             | 28.87                           | 0.754                           | 0.291        |
| GenScore(GatedGCN_0)           | 0.494        | 0.543        | 0.921                             | 0.952                             | 22.59                           | 0.52                            | 0.3          |
| GenScore(GatedGCN_1.0)         | 0.833        | 0.726        | 0.89                              | 0.905                             | 17.35                           | 0.544                           | 0.15         |
| GenScore(GatedGCN_ft_1.0)      | 0.824        | 0.709        | 0.926                             | 0.953                             | 26.41                           | 0.684                           | 0.205        |
| BioLM – Score <sub>base</sub>  | 0.496        | 0.545        | 0.934                             | <b>0.964</b>                      | 25.13                           | 0.585                           | <b>0.372</b> |
| BioLM – Score <sub>joint</sub> | <b>0.841</b> | <b>0.737</b> | 0.910                             | 0.931                             | 18.47                           | 0.591                           | 0.166        |
| BioLM – Score <sub>ft</sub>    | 0.809        | 0.681        | <b>0.943</b>                      | 0.957                             | <b>29.51</b>                    | <b>0.772</b>                    | 0.275        |

Table 2: Ablation study on different feature fusion methods

| Settings     | Methods    | Scoring      | Ranking      | Docking                    |                            | Screening                       |                                 |                                 |
|--------------|------------|--------------|--------------|----------------------------|----------------------------|---------------------------------|---------------------------------|---------------------------------|
|              |            | $R_p$        | $R_s$        | $SR_1$<br>(poses excluded) | $SR_1$<br>(poses included) | Forward Screening<br>$EF_{1\%}$ | Reverse screening<br>$SR_{1\%}$ | Reverse screening<br>$SR_{1\%}$ |
| $\alpha = 0$ | add        | 0.487        | 0.554        | 0.923                      | 0.958                      | 25.12                           | 0.561                           | 0.347                           |
|              | gated_add  | 0.465        | 0.546        | 0.923                      | 0.951                      | 24.47                           | 0.566                           | 0.357                           |
|              | cross_attn | 0.473        | 0.560        | 0.933                      | 0.951                      | 23.08                           | 0.579                           | 0.344                           |
|              | concat     | 0.496        | 0.545        | <b>0.934</b>               | <b>0.964</b>               | <b>25.13</b>                    | <b>0.585</b>                    | <b>0.372</b>                    |
| $\alpha = 1$ | add        | 0.821        | 0.732        | 0.902                      | 0.940                      | 17.53                           | 0.552                           | <b>0.225</b>                    |
|              | gated_add  | 0.827        | 0.739        | <b>0.916</b>               | <b>0.940</b>               | 18.32                           | <b>0.667</b>                    | 0.200                           |
|              | cross_attn | 0.833        | 0.735        | 0.891                      | 0.919                      | 16.46                           | 0.509                           | 0.154                           |
|              | concat     | <b>0.841</b> | <b>0.737</b> | 0.910                      | 0.931                      | <b>18.47</b>                    | 0.591                           | 0.166                           |
| finetune     | add        | <b>0.825</b> | 0.698        | 0.937                      | 0.958                      | 26.88                           | 0.737                           | 0.246                           |
|              | gated_add  | 0.809        | 0.688        | 0.930                      | 0.954                      | 29.04                           | 0.772                           | 0.273                           |
|              | cross_attn | 0.797        | <b>0.711</b> | 0.933                      | 0.954                      | 29.01                           | 0.772                           | 0.267                           |
|              | concat     | 0.809        | 0.681        | <b>0.943</b>               | <b>0.957</b>               | <b>29.51</b>                    | <b>0.772</b>                    | <b>0.275</b>                    |

Table 3: Ablation study on the contribution of protein and ligand language models

|              |                 | Scoring Ranking |       | Docking                           |                                   | Screening                       |                                 |                                 |
|--------------|-----------------|-----------------|-------|-----------------------------------|-----------------------------------|---------------------------------|---------------------------------|---------------------------------|
|              |                 | $R_p$           | $R_s$ | $SR_1$<br>(native poses excluded) | $SR_1$<br>(native poses included) | Forward Screening<br>$EF_{1\%}$ | Reverse screening<br>$SR_{1\%}$ | Reverse screening<br>$SR_{1\%}$ |
| $\alpha = 0$ | W/O protein LLM | 0.507           | 0.539 | 0.895                             | 0.93                              | 19.71                           | 0.483                           | 0.298                           |
|              | W/O ligand LLM  | 0.481           | 0.544 | 0.933                             | 0.958                             | 24.55                           | 0.596                           | 0.351                           |
|              | Full model      | 0.496           | 0.545 | 0.934                             | 0.964                             | 25.13                           | 0.585                           | 0.372                           |
| $\alpha = 1$ | W/O protein LLM | 0.842           | 0.732 | 0.874                             | 0.891                             | 15.21                           | 0.413                           | 0.132                           |
|              | W/O ligand LLM  | 0.837           | 0.725 | 0.902                             | 0.930                             | 19.4                            | 0.579                           | 0.144                           |
|              | Full model      | 0.841           | 0.737 | 0.910                             | 0.931                             | 18.47                           | 0.591                           | 0.166                           |
| finetune     | W/O protein LLM | 0.809           | 0.660 | 0.891                             | 0.919                             | 23.61                           | 0.569                           | 0.232                           |
|              | W/O ligand LLM  | 0.806           | 0.674 | 0.926                             | 0.954                             | 29.83                           | 0.737                           | 0.316                           |
|              | Full model      | 0.809           | 0.681 | 0.943                             | 0.957                             | 29.51                           | 0.772                           | 0.275                           |

Table 4: Node and edge features of the ligand graph.

| Feature                    | Dim. | Description                                                                                                                                  |
|----------------------------|------|----------------------------------------------------------------------------------------------------------------------------------------------|
| <i>Node Features</i>       |      |                                                                                                                                              |
| atom_type_one_hot          | 17   | One-hot encoding of atom type ([C, N, O, S, F, P, Cl, Br, I, B, Si, Fe, Zn, Cu, Mn, Mo, other])                                              |
| atom_degree_one_hot        | 7    | One-hot encoding of atom degree ([0, 1, 2, 3, 4, 5, 6])                                                                                      |
| atom_formal_charge         | 1    | Formal charge of the atom                                                                                                                    |
| atom_num_radical_electrons | 1    | Number of radical electrons                                                                                                                  |
| atom_hybridization_one_hot | 6    | One-hot encoding of hybridization type ([sp, sp <sup>2</sup> , sp <sup>3</sup> , sp <sup>3</sup> d, sp <sup>3</sup> d <sup>2</sup> , other]) |
| atom_is_aromatic           | 1    | Whether the atom is aromatic (Boolean)                                                                                                       |
| atom_total_num_H_one_hot   | 5    | One-hot encoding of the total number of hydrogen atoms ([0, 1, 2, 3, 4])                                                                     |
| atom_chirality_one_hot     | 3    | One-hot encoding of chirality center ([R, S, other])                                                                                         |
| <i>Edge Features</i>       |      |                                                                                                                                              |
| bond_type_one_hot          | 4    | One-hot encoding of bond type ([single, double, triple, aromatic])                                                                           |
| bond_is_conjugated         | 1    | Whether the bond is conjugated (Boolean)                                                                                                     |
| bond_is_in_ring            | 1    | Whether the bond is in a ring (Boolean)                                                                                                      |
| bond_stereo_one_hot        | 4    | One-hot encoding of stereochemistry ([none, any, Z-isomer, E-isomer])                                                                        |

Table 5: Node and edge features of the protein graph.

| Feature                  | Dim. | Description                                                                                                                                                                                               |
|--------------------------|------|-----------------------------------------------------------------------------------------------------------------------------------------------------------------------------------------------------------|
| <i>Node Features</i>     |      |                                                                                                                                                                                                           |
| residue_type_one_hot     | 32   | One-hot encoding of residue types, including amino acids ([GLY, ALA, VAL, LEU, ILE, PRO, PHE, TYR, TRP, SER, THR, CYS, MET, ASN, GLN, ASP, GLU, LYS, ARG, HIS]), metal ions, and other non-standard types |
| residue_self_distance    | 5    | Maximum and minimum distances between atoms within the residue (scaled by 0.1), and distances between specific atoms (e.g., $C\alpha$ -O, O-N, C-N)                                                       |
| residue_dihedral_angle   | 4    | Scaled residue dihedral angles (multiplied by 0.01), including $\phi$ , $\psi$ , $\omega$ , and $\chi_1$                                                                                                  |
| <i>Edge Features</i>     |      |                                                                                                                                                                                                           |
| residue_is_connected     | 1    | Whether two residues are directly connected via a covalent bond (Boolean)                                                                                                                                 |
| residue_CA_distance      | 1    | Scaled distance between $C\alpha$ atoms of two residues (multiplied by 0.1)                                                                                                                               |
| residue_center_distance  | 1    | Scaled distance between the centroids of two residues (multiplied by 0.1)                                                                                                                                 |
| residue_maximum_distance | 2    | Scaled maximum and minimum atomic distances between two residues (multiplied by 0.1)                                                                                                                      |

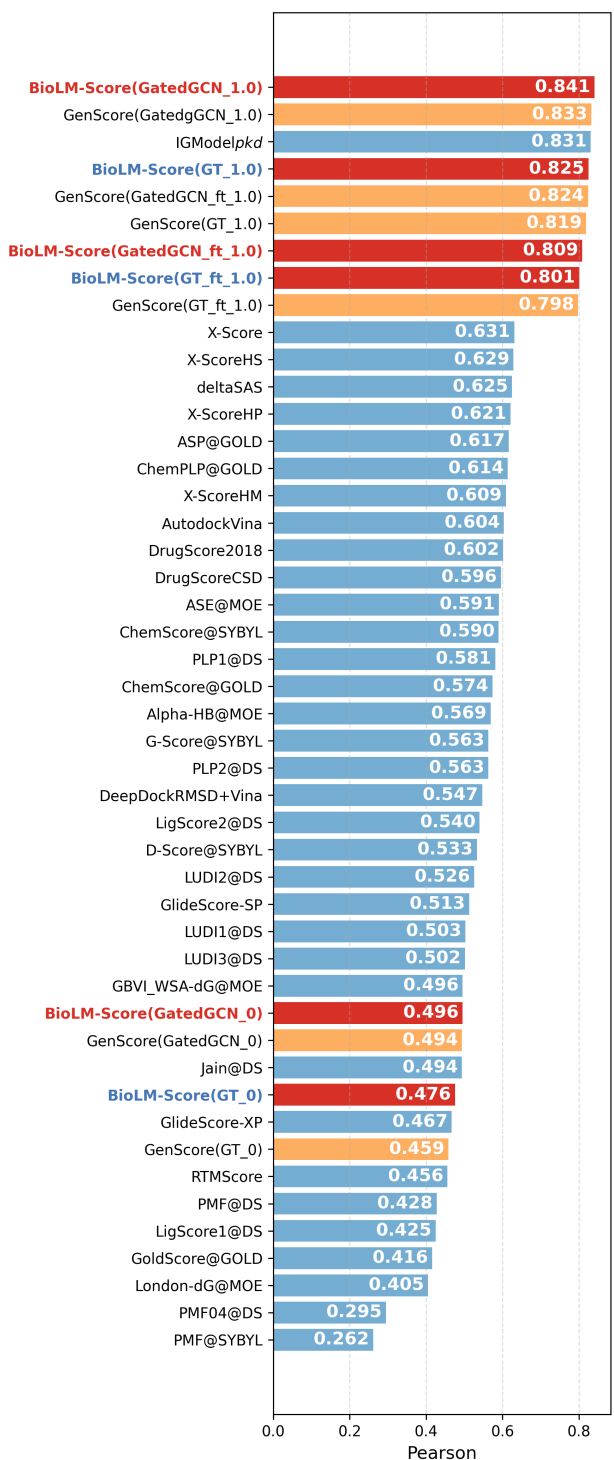

Figure 1: Evaluation of scoring power on the CASF-2016 benchmark. The figure shows the Pearson correlation coefficient ( $R_p$ ) ranking compared with other scoring functions.

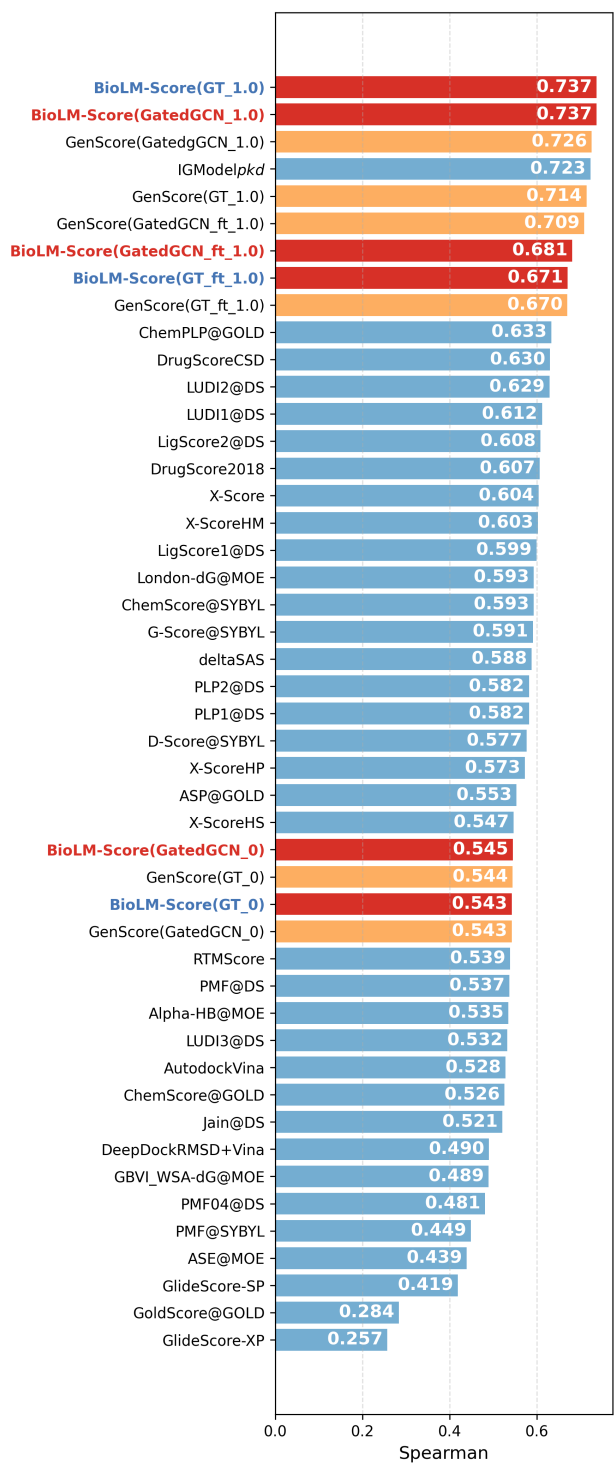

Figure 2: Evaluation of ranking power on the CASF-2016 benchmark. The figure shows the Spearman correlation coefficient ( $R_s$ ) ranking compared with other scoring functions.

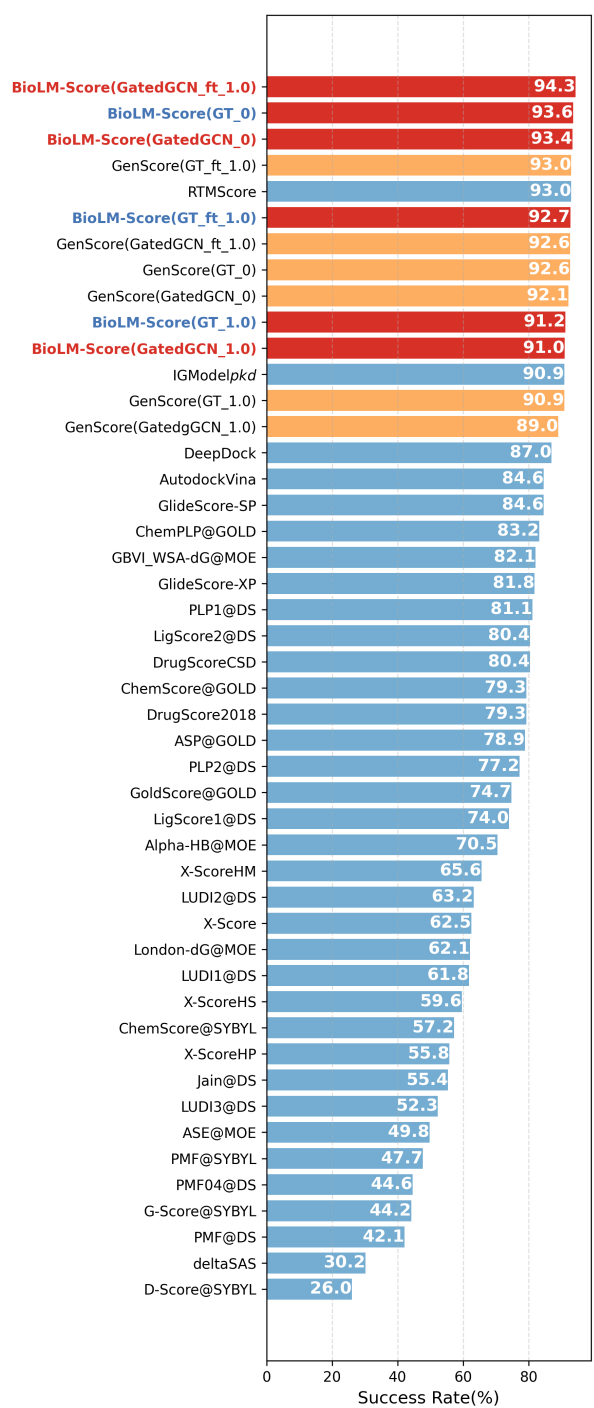

(a) With crystallized poses

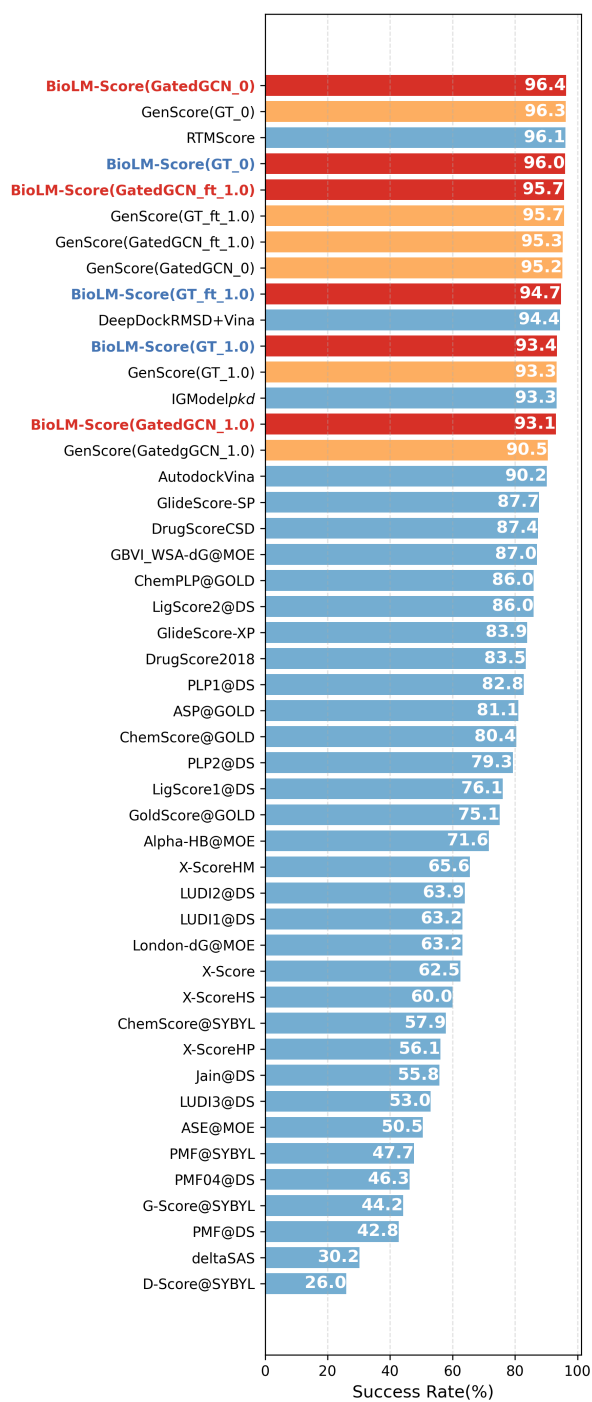

(b) Without crystallized poses

Figure 3: Evaluation of docking power on the CASF-2016 benchmark based on success rates at the top 1. (a) Including crystallized poses in the test set; (b) Excluding crystallized poses in the test set.

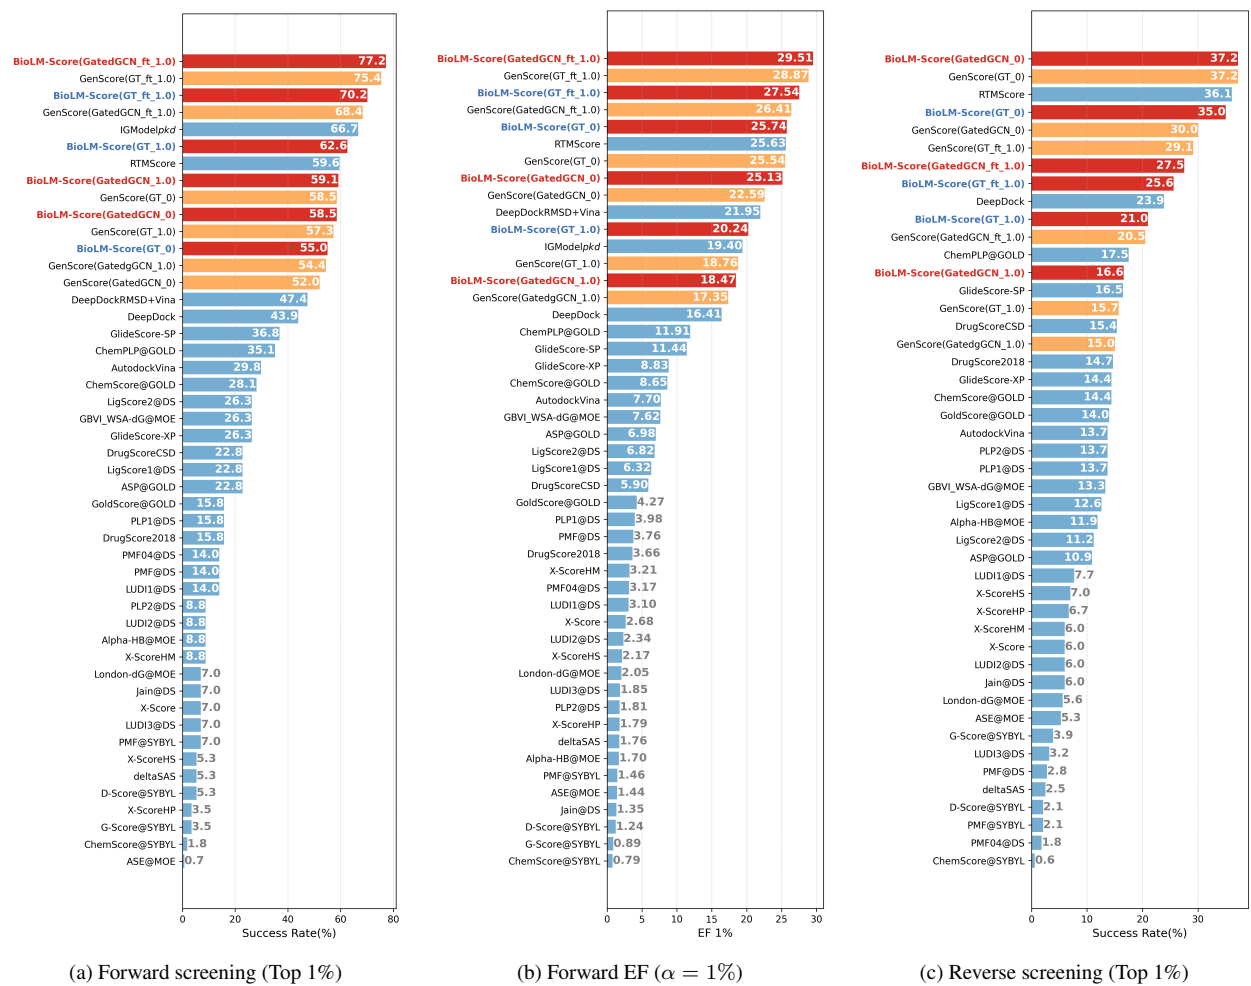

Figure 4: Evaluation of screening power on the CASF-2016 benchmark. (a) Top 1% success rate in forward screening; (b) Enrichment factor ( $\alpha = 1\%$ ) in forward screening; (c) Top 1% success rate in reverse screening.
